# Supplementary material for: Active Preference Learning over Latent Preference Archetypes for Many-Objective Bayesian Optimization
Source: arXiv:2603.28410 source file (2026-08-27)
Supplement: Supplementary file 1 [file Supplementary.tex]

\section{Theoretical Proofs}
In this section, we detail the proof of the theorem stated in the main paper. We state model setup and assumptions. Then we prove Lipschitz properties of the utility. Further, we discuss surrogate mismatch bound. Further, we combine all the pieces for the regret decomposition theorem. 

\subsection*{Model Assumptions}
We consider $m$ objectives to be \emph{minimized}. For any outcome vector $y\in\mathbb R^m$
and weights $w\in\Delta^{m-1}$, define the Chebyshev utility
\begin{equation}
\label{eq:neg-cheb}
U(y,w)\coloneqq -\min_{1\le j\le m}\frac{y_j}{w_j}.
\end{equation}
Thus larger utility is preferred. We assume all weights are bounded away from the simplex
boundary: there exists $c_w>0$ such that $w_j\ge c_w$ for all $j$ for every true archetype
$w_k^\star$ and every estimated archetype $\hat w_{k,t}$.

Let the true latent preferences be a mixture of $K_\star$ archetypes with weights
$\eta^\star\in\Delta^{K_\star-1}$ and archetypes $\{w_k^\star\}_{k=1}^{K_\star}\subset\Delta^{m-1}$.
Define the true mixture utility at design $x\in\mathcal X$ by
\begin{equation}
\label{eq:true-mix-util}
\mathcal U^\star(x)\coloneqq \sum_{k=1}^{K_\star}\eta_k^\star\,U\!\big(f(x),w_k^\star\big),
\qquad
\mathcal U^\star \coloneqq \sup_{x\in\mathcal X} \mathcal U^\star(x).
\end{equation}

The algorithm fits one GP per objective $f_j$ and maintains posterior mean
$\mu_{t-1,j}(x)$ and standard deviation $\sigma_{t-1,j}(x)$ after $t-1$ evaluations.
Let $\mu_{t-1}(x)\in\mathbb R^m$ be the vector of means. At round $t$, the preference model outputs estimates $\hat\eta_t\in\Delta^{K-1}$
and $\{\hat w_{k,t}\}_{k=1}^K$. Define the surrogate mixture utility used for acquisition
\begin{equation}
\label{eq:surrogate-mix-util}
\widehat{\mathcal U}_t(x)\coloneqq \sum_{k=1}^{K}\hat\eta_{k,t}\,U\!\big(\mu_{t-1}(x),\hat w_{k,t}\big).
\end{equation}
Assume the selected point $x_t$ is $\varepsilon_t$-optimal for the surrogate:
\begin{equation}
\label{eq:eps-opt}
\widehat{\mathcal U}_t(x_t)\ge \sup_{x\in\mathcal X}\widehat{\mathcal U}_t(x)-\varepsilon_t.
\end{equation}

\begin{assumption}[Bounded Objectives]
$\|f(x)\|_\infty \le B_y \quad \forall x\in\mathcal X$
\end{assumption}

\paragraph{Alignment and estimation errors}
Let $\pi_t$ be a permutation (e.g., Hungarian matching) aligning estimated archetypes
to true archetypes. Pad $\eta^\star$ with zeros if $K>K_\star$. Define
\begin{equation}
\label{eq:deltas}
\Delta_t^{w}\coloneqq \sum_{k=1}^{K_\star}\eta_k^\star\,
\|\hat w_{\pi_t(k),t}-w_k^\star\|_1,
\qquad
\Delta_t^{\eta}\coloneqq \|\hat\eta_t-\eta^\star\|_1.
\end{equation}

\begin{lemma}[Lipschitzness of Chebyshev utility]
\label{lem:lipschitz-neg-cheb}
Let $U$ be as in \eqref{eq:neg-cheb} and assume $w_j,w'_j\ge c_w>0$ for all $j$.
Then for any $y,y'\in\mathbb R^m$ and any such $w,w'\in\Delta^{m-1}$,
\begin{align}
\big|U(y,w)-U(y',w)\big|
&\le \frac{1}{c_w}\,\|y-y'\|_\infty,
\label{eq:Lip-y}\\
\big|U(y,w)-U(y,w')\big|
&\le \frac{\|y\|_\infty}{c_w^2}\,\|w-w'\|_1.
\label{eq:Lip-w}
\end{align}
\end{lemma}

\begin{proof}
For \eqref{eq:Lip-y}, fix $w$ and define $g_j(y)\coloneqq -y_j/w_j$. Each $g_j$ is
$(1/c_w)$-Lipschitz under $\|\cdot\|_\infty$ because
$|g_j(y)-g_j(y')|=|y_j-y'_j|/w_j\le \|y-y'\|_\infty/c_w$.
Since $U(y,w)=\min_j g_j(y)$ is the pointwise minimum of $(1/c_w)$-Lipschitz functions,
it is itself $(1/c_w)$-Lipschitz, proving \eqref{eq:Lip-y}.

For \eqref{eq:Lip-w}, fix $y$ and write $U(y,w)=\min_j h_j(w)$ with
$h_j(w)\coloneqq -y_j/w_j$. For any $j$,
\[
|h_j(w)-h_j(w')|
=
|y_j|\left|\frac{1}{w_j}-\frac{1}{w'_j}\right|
=
\frac{|y_j|\,|w_j-w'_j|}{w_jw'_j}
\le
\frac{\|y\|_\infty}{c_w^2}\,|w_j-w'_j|.
\]
Therefore
\[
|U(y,w)-U(y,w')|
\le
\max_j |h_j(w)-h_j(w')|
\le
\frac{\|y\|_\infty}{c_w^2}\max_j|w_j-w'_j|
\le
\frac{\|y\|_\infty}{c_w^2}\|w-w'\|_1,
\]
which proves \eqref{eq:Lip-w}.
\end{proof}

\subsection*{GP confidence}

We use a standard high-probability confidence bound for each objective GP.
Assume sub-Gaussian observation noise and conditions under which the standard GP-UCB
confidence event holds for each objective (e.g., \cite{srinivas2010gaussian}).

\begin{assumption}[Per-objective GP confidence event]
\label{ass:gp-conf}
There exists a nondecreasing sequence $\{\beta_t\}$ such that with probability at least
$1-\delta$, simultaneously for all $t\ge 1$, all $x\in\mathcal X$, and all $j\in\{1,\dots,m\}$,
\begin{equation}
\label{eq:gp-per-obj}
|f_j(x)-\mu_{t-1,j}(x)|
\le
\sqrt{\beta_t}\,\sigma_{t-1,j}(x).
\end{equation}
\end{assumption}

Under \eqref{eq:gp-per-obj}, we have for all $x$,
\begin{equation}
\label{eq:vector-gp}
\|f(x)-\mu_{t-1}(x)\|_\infty
\le
\sqrt{\beta_t}\,\|\sigma_{t-1}(x)\|_\infty.
\end{equation}

\subsection*{Main result: simple regret decomposition}

Define the simple regret under the \emph{true} mixture utility:
\begin{equation}
\label{eq:simple-regret}
R_T \coloneqq \mathcal U^\star - \max_{t\le T}\mathcal U^\star(x_t).
\end{equation}

\begin{theorem}[Simple regret decomposition]
\label{thm:regret-decomp-safe}
On the GP confidence event in Assumption~\ref{ass:gp-conf}, for any $T\ge 1$,
\begin{equation}
\label{eq:regret-decomp}
R_T
\le
\underbrace{\frac{2}{c_w}\min_{t\le T}\|f(x_t)-\mu_{t-1}(x_t)\|_\infty}_{\textnormal{objective GP term}}
+
\underbrace{\frac{2B_y}{c_w^2}\min_{t\le T}\Delta_t^{w}}_{\textnormal{archetype error}}
+
\underbrace{\frac{2B_y}{c_w}\min_{t\le T}\Delta_t^{\eta}}_{\textnormal{mixture-weight error}}
+
\underbrace{\max_{t\le T}\varepsilon_t}_{\textnormal{surrogate maximization}}.
\end{equation}
Moreover, still on the same event, the objective GP term admits an existence-type rate:
\begin{equation}
\label{eq:gp-rate-existence}
\min_{t\le T}\|f(x_t)-\mu_{t-1}(x_t)\|_\infty
\le
\frac{1}{T}\sum_{t=1}^T \|f(x_t)-\mu_{t-1}(x_t)\|_\infty
\;\lesssim\;
\sqrt{\frac{\beta_T\,\gamma_T}{T}},
\end{equation}
where $\gamma_T$ is a (max) information-gain term for the objective GPs (taking the maximum
over objectives if kernels differ), and $\lesssim$ hides constants depending only on the kernels and noise.
\end{theorem}

\begin{proof}
Let $x^\star\in\arg\max_{x\in\mathcal X}\mathcal U^\star(x)$. Fix any round $t\ge 1$.
Add and subtract the surrogate utility \eqref{eq:surrogate-mix-util} at $x^\star$ and $x_t$:
\begin{align}
\mathcal U^\star(x^\star)-\mathcal U^\star(x_t)
&=
\big(\mathcal U^\star(x^\star)-\widehat{\mathcal U}_t(x^\star)\big)
+
\big(\widehat{\mathcal U}_t(x^\star)-\widehat{\mathcal U}_t(x_t)\big)
+
\big(\widehat{\mathcal U}_t(x_t)-\mathcal U^\star(x_t)\big).
\label{eq:three-brackets}
\end{align}
By $\varepsilon_t$-optimality \eqref{eq:eps-opt}, the middle term is at most $\varepsilon_t$.
Therefore,
\begin{equation}
\label{eq:two-mismatch}
\mathcal U^\star(x^\star)-\mathcal U^\star(x_t)
\le
\big|\mathcal U^\star(x^\star)-\widehat{\mathcal U}_t(x^\star)\big|
+
\big|\mathcal U^\star(x_t)-\widehat{\mathcal U}_t(x_t)\big|
+
\varepsilon_t.
\end{equation}
It remains to bound $|\mathcal U^\star(x)-\widehat{\mathcal U}_t(x)|$ for a generic $x$.

\textbf{Step 1: (Decomposition)}
Using \eqref{eq:true-mix-util} and \eqref{eq:surrogate-mix-util},
\[
\mathcal U^\star(x)-\widehat{\mathcal U}_t(x)
=
\sum_{k=1}^{K_\star}\eta_k^\star U(f(x),w_k^\star)
-
\sum_{k=1}^{K}\hat\eta_{k,t} U(\mu_{t-1}(x),\hat w_{k,t}).
\]
Insert and subtract $\sum_{k=1}^{K_\star}\eta_k^\star U(\mu_{t-1}(x),w_k^\star)$ and
$\sum_{k=1}^{K_\star}\eta_k^\star U(\mu_{t-1}(x),\hat w_{\pi_t(k),t})$, then apply triangle inequality:
\begin{align}
\big|\mathcal U^\star(x)-\widehat{\mathcal U}_t(x)\big|
&\le
\sum_{k=1}^{K_\star}\eta_k^\star
\big|U(f(x),w_k^\star)-U(\mu_{t-1}(x),w_k^\star)\big|
\notag\\
&\quad+
\sum_{k=1}^{K_\star}\eta_k^\star
\big|U(\mu_{t-1}(x),w_k^\star)-U(\mu_{t-1}(x),\hat w_{\pi_t(k),t})\big|
\notag\\
&\quad+
\left|\sum_{k=1}^{K}(\eta_k^\star-\hat\eta_{k,t})\,U(\mu_{t-1}(x),\hat w_{k,t})\right|.
\label{eq:mismatch-decomp}
\end{align}

\textbf{Step 2: (Bounding terms using Lemma~\ref{lem:lipschitz-neg-cheb})}
For the first line, apply Lipschitzness in $y$ \eqref{eq:Lip-y}:
\[
\big|U(f(x),w_k^\star)-U(\mu_{t-1}(x),w_k^\star)\big|
\le
\frac{1}{c_w}\,\|f(x)-\mu_{t-1}(x)\|_\infty.
\]
Summing over $k$ with weights $\eta_k^\star$ gives
\begin{equation}
\label{eq:termA}
\sum_{k=1}^{K_\star}\eta_k^\star
\big|U(f(x),w_k^\star)-U(\mu_{t-1}(x),w_k^\star)\big|
\le
\frac{1}{c_w}\,\|f(x)-\mu_{t-1}(x)\|_\infty.
\end{equation}

For the second line, apply Lipschitzness in $w$ \eqref{eq:Lip-w} with $\| \mu_{t-1}(x)\|_\infty\le B_y$:
\[
\big|U(\mu_{t-1}(x),w_k^\star)-U(\mu_{t-1}(x),\hat w_{\pi_t(k),t})\big|
\le
\frac{B_y}{c_w^2}\,\|\hat w_{\pi_t(k),t}-w_k^\star\|_1.
\]
Thus the second line is bounded by $(B_y/c_w^2)\Delta_t^w$.

For the third line, use $|U(\mu_{t-1}(x),\hat w_{k,t})|
\le \|\mu_{t-1}(x)\|_\infty/c_w \le B_y/c_w$ to obtain
\begin{equation}
\label{eq:termC}
\left|\sum_{k=1}^{K}(\eta_k^\star-\hat\eta_{k,t})\,U(\mu_{t-1}(x),\hat w_{k,t})\right|
\le
\frac{B_y}{c_w}\,\|\hat\eta_t-\eta^\star\|_1
=
\frac{B_y}{c_w}\,\Delta_t^\eta.
\end{equation}

Combining \eqref{eq:mismatch-decomp}, \eqref{eq:termA} and \eqref{eq:termC}, we conclude that for all $x$,
\begin{equation}
\label{eq:mismatch-bound-final}
\big|\mathcal U^\star(x)-\widehat{\mathcal U}_t(x)\big|
\le
\frac{1}{c_w}\,\|f(x)-\mu_{t-1}(x)\|_\infty
+
\frac{B_y}{c_w^2}\Delta_t^w
+
\frac{B_y}{c_w}\Delta_t^\eta.
\end{equation}

\textbf{Step 3: (Convert to simple regret)}
Apply \eqref{eq:mismatch-bound-final} at $x=x^\star$ and $x=x_t$ in \eqref{eq:two-mismatch}:
\begin{align}
\mathcal U^\star(x^\star)-\mathcal U^\star(x_t)
&\le
\frac{1}{c_w}\Big(\|f(x^\star)-\mu_{t-1}(x^\star)\|_\infty + \|f(x_t)-\mu_{t-1}(x_t)\|_\infty\Big)
\notag\\
&\quad+
\frac{2B_y}{c_w^2}\Delta_t^w
+
\frac{2B_y}{c_w}\Delta_t^\eta
+
\varepsilon_t.
\label{eq:per-round-bound}
\end{align}

Now take the minimum over $t\le T$ on the right-hand side. Since
$R_T = \min_{t\le T}\big(\mathcal U^\star(x^\star)-\mathcal U^\star(x_t)\big)$ and
$\max_{t\le T}\varepsilon_t$ upper bounds $\varepsilon_t$, we obtain \eqref{eq:regret-decomp}. On the GP confidence event \eqref{eq:gp-per-obj}, the bound
\[
\|f(x)-\mu_{t-1}(x)\|_\infty
\le
\sqrt{\beta_t}\,\|\sigma_{t-1}(x)\|_\infty
\]
holds for all $x\in\mathcal X$, including $x^\star$.

\paragraph{Step 4: (Existence-type GP rate)}
On the confidence event \eqref{eq:gp-per-obj},
\[
\|f(x_t)-\mu_{t-1}(x_t)\|_\infty
\le
\sqrt{\beta_t}\,\|\sigma_{t-1}(x_t)\|_\infty
\le
\sqrt{\beta_T}\,\|\sigma_{t-1}(x_t)\|_\infty.
\]
Under standard variance-sum bounds for GP regression (e.g., Lemma X),
\[
\sum_{t=1}^T \|\sigma_{t-1}(x_t)\|_\infty^2
\le C\,\gamma_T,
\]
which implies
\[
\min_{t\le T} \|\sigma_{t-1}(x_t)\|_\infty
\le
\frac1T\sum_{t=1}^T \|\sigma_{t-1}(x_t)\|_\infty
\le
\sqrt{\frac{C\,\gamma_T}{T}}.
\]

\end{proof}

\section{Additional Experimental Details }

\subsection{Simulated Datasets}
We use well-known MOO benchmarks for our experimental setup, called DTLZ \cite{deb2005scalable} and WFG suite \cite{huband2005scalable}. We evaluate on DTLZ2 with \(L=6\) objectives and \(d=7\) decision variables
(minimization), search space \([0,1]^d\). At each design \(\mathbf x\in[0,1]^7\) we observe
\(\mathbf y=\mathbf f(\mathbf x)\). We also use WFG9 with $L=8$ objectives and $d=34$ decision variables. Following common practice, we set the WFG position parameter $k=2(L-1)=14$ and distance parameter $l=20$ so $d=k+l$. Variables are scaled to $[0,1]$ and all objectives are minimized. A design
$\mathbf x\!\in\![0,1]^d$ evaluates to an objective vector
$\mathbf y=\mathbf f(\mathbf x)\in\mathbb{R}^8$. WFG9 induces challenging biases and mixed separability, making it a stronger testbed for query policies.

To construct distinct but overlapping preference archetypes, we partition the objectives into disjoint groups and assign structured weight vectors. For the DTLZ suite (\(L=6\)), we define three groups
$
\mathcal G_1=\{0,1\}, \quad 
\mathcal G_2=\{2,3\}, \quad 
\mathcal G_3=\{4,5\}$ while for the WFG suite (\(L=8\)) we define four groups
$
\mathcal G_1=\{0,1\}, \;
\mathcal G_2=\{2,3\}, \;
\mathcal G_3=\{4,5\}, \;
\mathcal G_4=\{6,7\}.
$
Each mode allocates \(80\%\) of its total mass uniformly across its dominant group \(\mathcal G_k\) and distributes the remaining \(20\%\) uniformly over the other objectives. The resulting vector is renormalized to ensure \(\mathbf w_k \in \Delta^{L-1}\). This construction yields clearly separated trade-off profiles while maintaining nonzero sensitivity to all objectives.

Let \(Z_t \in \{1,\dots,K\}\) denote the active preference mode at query \(t\). Under an iid context regime, each query is generated independently according to a fixed mixture \(Z_t \sim \mathrm{Categorical}(\eta^\star)\), with \(\eta^\star=(0.5,0.3,0.2)\) for DTLZ and \(\eta^\star=\{(0.60,0.25,0.15,0.10)\), \(0.4, 0.3, 0.3, 0.1\)\} for WFG. Under a persistent context regime, the mode evolves according to a stay-or-resample process with persistence parameter \(\rho \in [0,1)\). The initial mode is drawn as \(Z_1 \sim \mathrm{Categorical}(\eta^\star)\), and at each subsequent query the mode remains unchanged with probability \(\rho\) and is resampled from \(\mathrm{Categorical}(\eta^\star)\) with probability \(1-\rho\). The expected run length within a single mode is \(1/(1-\rho)\), and the expected number of switches over \(T\) queries is \((1-\rho)(T-1)\).

\subsection{Real-World: PET Process Design}

We evaluate the proposed framework on a real-world multi-objective process design problem for polyethylene terephthalate (PET) production. The dataset comprises 10{,}000 previously evaluated process designs. Each design is represented by a 12-dimensional continuous decision vector $\mathbf x \in \mathbb{R}^{12}$ corresponding to operating and design parameters such as temperatures, pressures, residence times, and feed ratios. Each variable is bounded within physically meaningful limits and normalized to $[0,1]$ for modeling purposes. For each design, we consider $L=7$ objectives consisting of Return on Investment (ROI), life-Cycle Assessment (LCA) indicators, including global warming potential (GWP), terrestrial acidification, water consumption, fossil depletion, surplus ore, and human toxicity. 

To model heterogeneous chemist preferences, we construct $K=3$ archetypal weight vectors $\mathbf w_k \in \Delta^{6}$ that parameterize the Chebyshev scalarization. Objectives are grouped semantically Type A (Economic) which emphasizes on ROI, Type B (Environmental) which cares about environmental LCA indicators, Type C (Health-focused) which stresses on toxicity-related indicators. Each archetype allocates $80\%$ of its mass to its dominant objective group and distributes the remaining $20\%$ across the other objectives, followed by renormalization. This construction yields clearly distinct yet overlapping trade-off profiles that reflect plausible real-world stakeholder types. At each comparison step $t$, a latent mode variable $Z_t \in \{1,2,3\}$ determines which archetype governs the user's decision. Modes are sampled from a categorical distribution with mixture weights $\eta = [0.40,\,0.35,\,0.25]$ representing the population-level prevalence of economic, environmental, and health-oriented chemists. The parameter $\eta$ therefore controls the global heterogeneity across users. To capture temporal consistency, we adopt a sticky gating process with persistence parameter $\rho \in [0,1)$. The initial mode is drawn from $\mathrm{Categorical}(\eta)$, and at each subsequent step the mode remains unchanged with probability $\rho$ and is resampled from $\eta$ with probability $1-\rho$. In our experiments we set $\rho = 0.8$, implying strong short-term consistency in preferences. The preferences are generated using the same method as mentioned in the simulated settings. 

\subsection{Interaction Contexts}

We evaluate preference learning under the following two feedback regimes.

\paragraph{Persistent context}
A latent archetype $z_t \in \{1,\dots,K_\star\}$ evolves with temporal inertia. At round $t$,
\[
z_t =
\begin{cases}
z_{t-1}, & \text{with probability } \rho,\\
\mathrm{Categorical}(\eta^\star), & \text{with probability } 1-\rho,
\end{cases}
\]
where $\eta^\star \in \Delta^{K_\star-1}$ are the true mixture weights and 
$\rho \in [0,1)$ controls stickiness. The initial archetype $z_1$ is sampled from 
$\mathrm{Categorical}(\eta^\star)$. Conditional on $z_t = k$, pairwise feedback is generated using utility 
$U\!\big(f(x), w_k^\star\big)$ under a probit likelihood. This regime induces temporally coherent feedback and facilitates identification and refinement of active archetypes.

\paragraph{I.i.d. context.}
At each round,
\[
z_t \sim \mathrm{Categorical}(\eta^\star),
\]
independently across $t$. Each comparison is therefore generated from an independently sampled archetype, removing temporal continuity. This regime is more challenging for mode identification, as archetype switches occur randomly and minority modes are observed less frequently in expectation.

All methods are evaluated under both regimes using identical seeds and evaluation budgets.

\subsection{Implementation Details:} 
We conduct our experiments on two simulated WFG and DTLZ and one real-world dataset. We consider stickiness parameter to be $0.5$ for both DTLZ and WFG dataset. While simulation of clusters, we consider \(\eta^\star=(0.5,0.3,0.2)\) for DTLZ,  $\eta^\star=(0.50,\,0.25,\,0.15,\,0.10)$ for WFG suite and \(\eta^\star=(0.40, 0.35, 0.25)\) for Chemistry Process Design. 
We use Python 3.12 with JAX/JAXlib, NumPyro, Optuna, and GPy. Each objective is modeled with an independent GP (RBF kernel); for synthetic/WFG experiments GPs are refit every 3 iterations with bounded noise and data-adaptive bounds on variance and lengthscale, whereas for chemistry experiments pretrained GP surrogates are loaded and queried. Preferences follow a probit likelihood with noise $u_{\sigma}$ is set to 0.02 for WFG/DTLZ dataset and 0.1 for PET process design dataset. Heterogeneous preferences are modeled via a truncated stick-breaking DP mixture with preknown K components and variational inference using SVI (Adam lr=1e-3, 500 updates per iteration). Preference queries are selected from pairs of previously observed outcomes using entropy/MI-based criteria (modes: clusterless/inter/intra/hybrid). Candidate points are proposed by MC expected improvement with 12 samples and 10 L-BFGS-B restarts. All randomness (initial seeds, EI samples, query subsampling, sticky archetype gating, and variational initialization) is controlled by a single run seed. All methods share an identical initial seed dataset injected into Optuna. Simple regret uses a common reference $U^{*}$ estimated by random search with 500 samples (saved and reused). We report mean ± std across 3 runs (different run seeds).

\subsection{Additional Metrics} 1) \textbf{Mixture-weight calibration} We compare the posterior mean mixture weights $\hat{\boldsymbol{\eta}}$ to the ground-truth weights $\boldsymbol{\eta}^\star$ projected via the same alignment (bar plot), and track $\mathrm{KL}\!\left(\boldsymbol{\eta}^\star \,\|\, \tilde{\boldsymbol{\eta}}\right)$ over iterations (lower is better). Blue-only mass indicates spurious modes, orange-only mass indicates missed modes. 2) \textbf{Errors of inferred preferences:} Errors of inferred preferences relative to single reference $w_{true}$: mixture-mean $\mid \mid w_{true} - \sum_k \eta_k \bar{w}_k \mid \mid_1$, MAP-cluster $\mid \mid w_{true} - \bar{w}_{k^*}\mid \mid$ with $k^* = \arg \max_k \eta_k$ and expected $\sum_k \eta_k  \mid \mid w_{true} - \bar{w}_k \mid \mid_1$. Lower is better.

\begin{table}[t]
\centering
\small
\begin{tabular}{ll}
\toprule
Symbol & Meaning \\
\midrule
$L$ & number of objectives \\
$K$ & truncation level (max modes) \\
$\ell$ & objective index \\
$k$ & preference mode index \\
$\mathbf w_k$ & weight vector for mode $k$ \\
$\eta_k$ & mixture weight of mode $k$ \\
$r_i$ & latent mode for comparison $i$ \\
$\sigma_u$ & preference noise parameter \\
\bottomrule
\end{tabular}
\caption{Notation summary.}
\end{table}

\section{Results and Analysis}

Figure \ref{fig:metric3} shows mixture-weight calibration for DTLZ2 dataset. We can observe here that in random plot blue mass is concentrated on one index and a big orange bar has almost no blue in several panels, hence indicating towards mode collapse. In intra-cluster, we can see that it is focussing on one cluster's shape since it doesnt tru to calibrate $\eta$. In the inter-query plot, we can see separate modes, and  more blue bars are lining up with orange bars where orange bars indicate projected true $\eta^*$. 

Figure \ref{fig:metric4} shows errors of inferred preferences for persistent user for DTLZ2 dataset for clusterless and inter-query modes. we can observe that mixture-mean/expected errors creep up, and MAP worsens. That's consistent with uncertainty sampling under collapsed scalarizer. Since clusterless mode ignores disagreement between archetypes, it chases high entropy and can drift away from the true mode. In the plot of inter-query, we can observe that the expected and mixture-mean errors decline clearly. Here, we can also note that MAP improves more slowly. It shows how inter queries look for identity first and tend to cut mixture confusion early. 

\begin{figure*}
\centering
% First row
\begin{subfigure}{0.33\textwidth}
  \includegraphics[width=\linewidth]{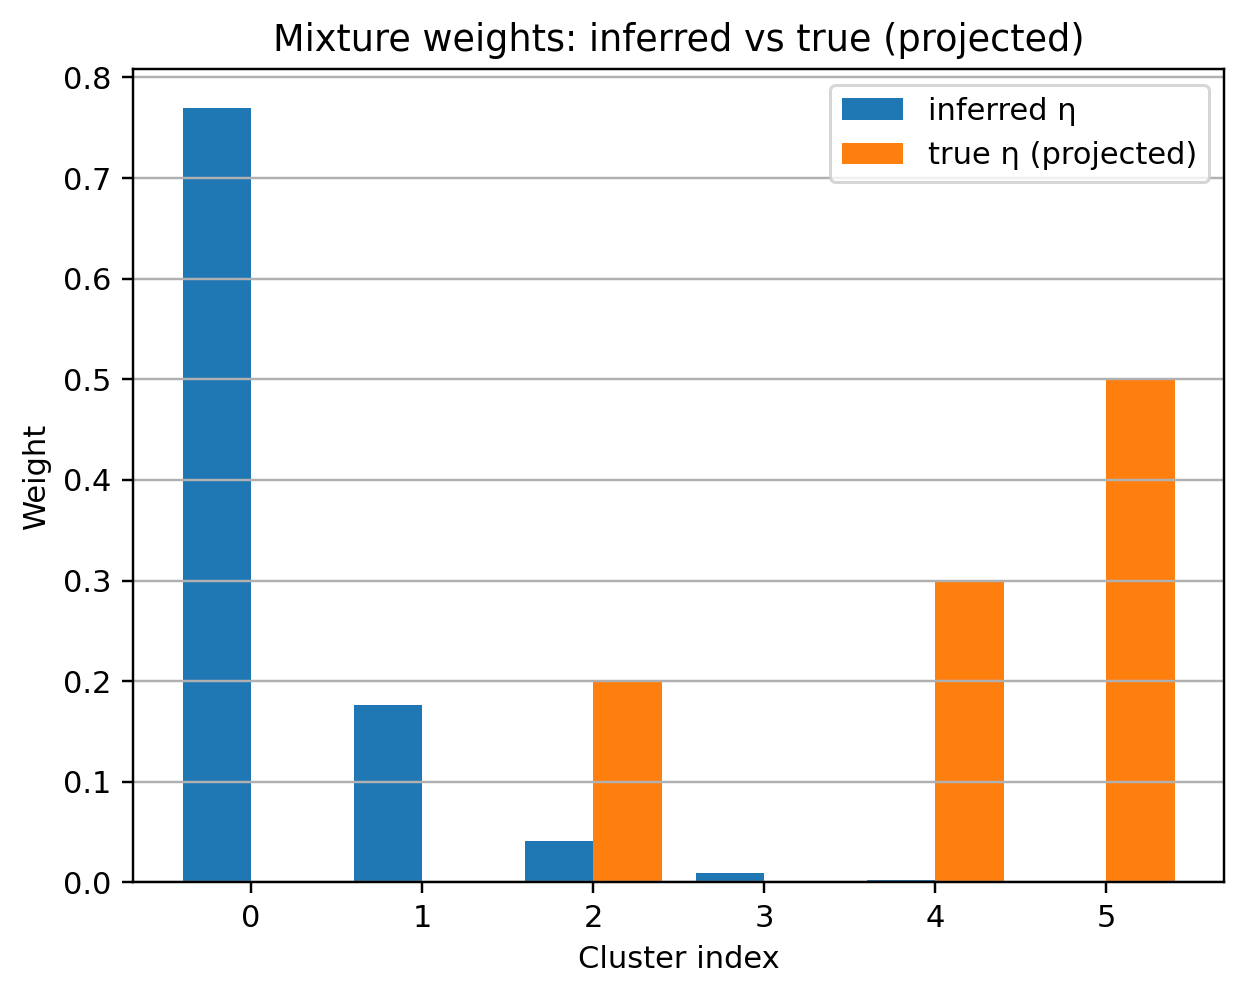}
  \caption{Random}
\end{subfigure}\hfill
\begin{subfigure}{0.33\textwidth}
  \includegraphics[width=\linewidth]{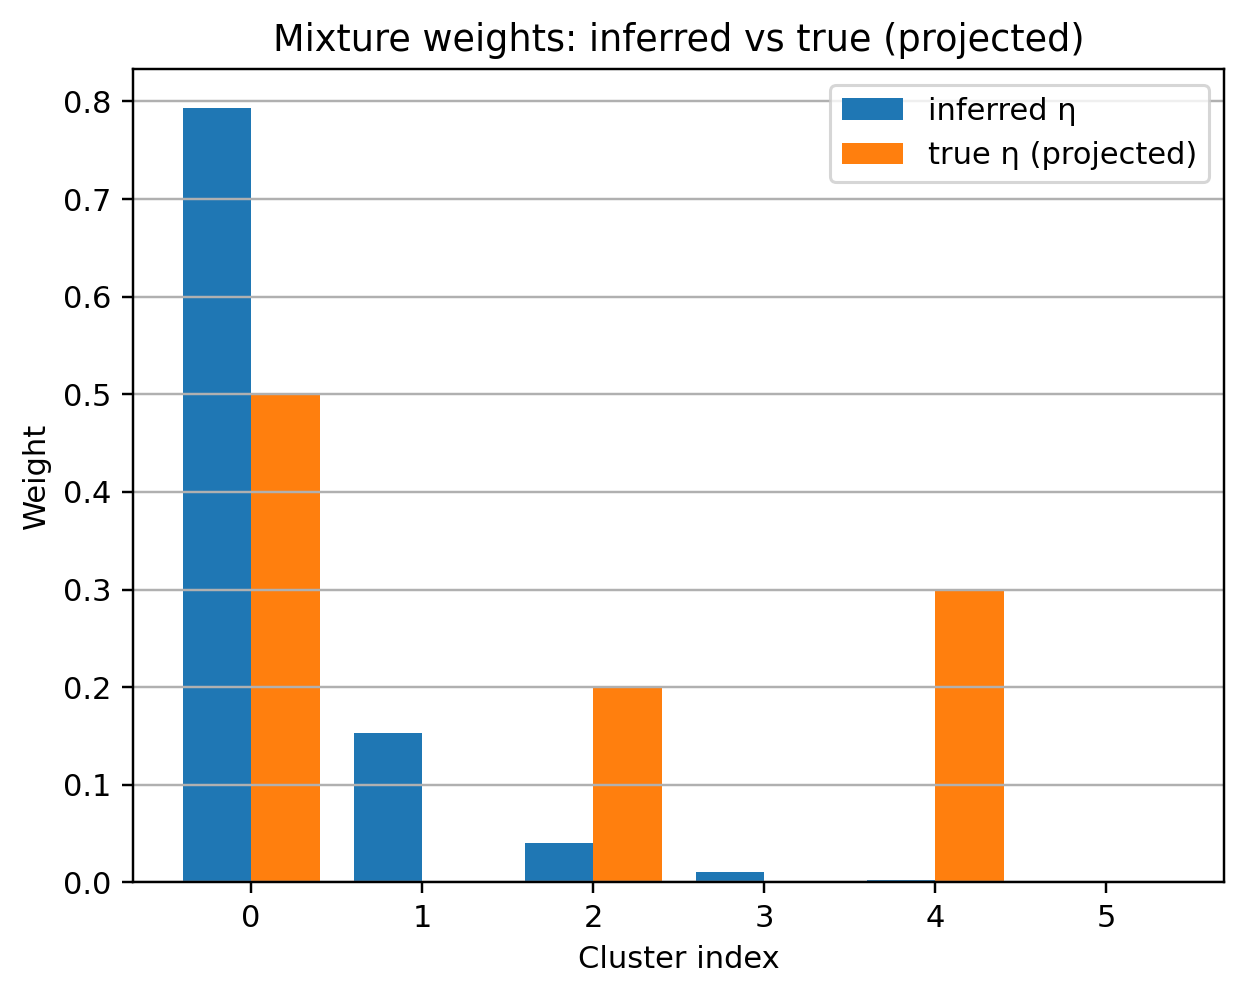}
  \caption{Intra}
\end{subfigure}\hfill
\begin{subfigure}{0.33\textwidth}
  \includegraphics[width=\linewidth]{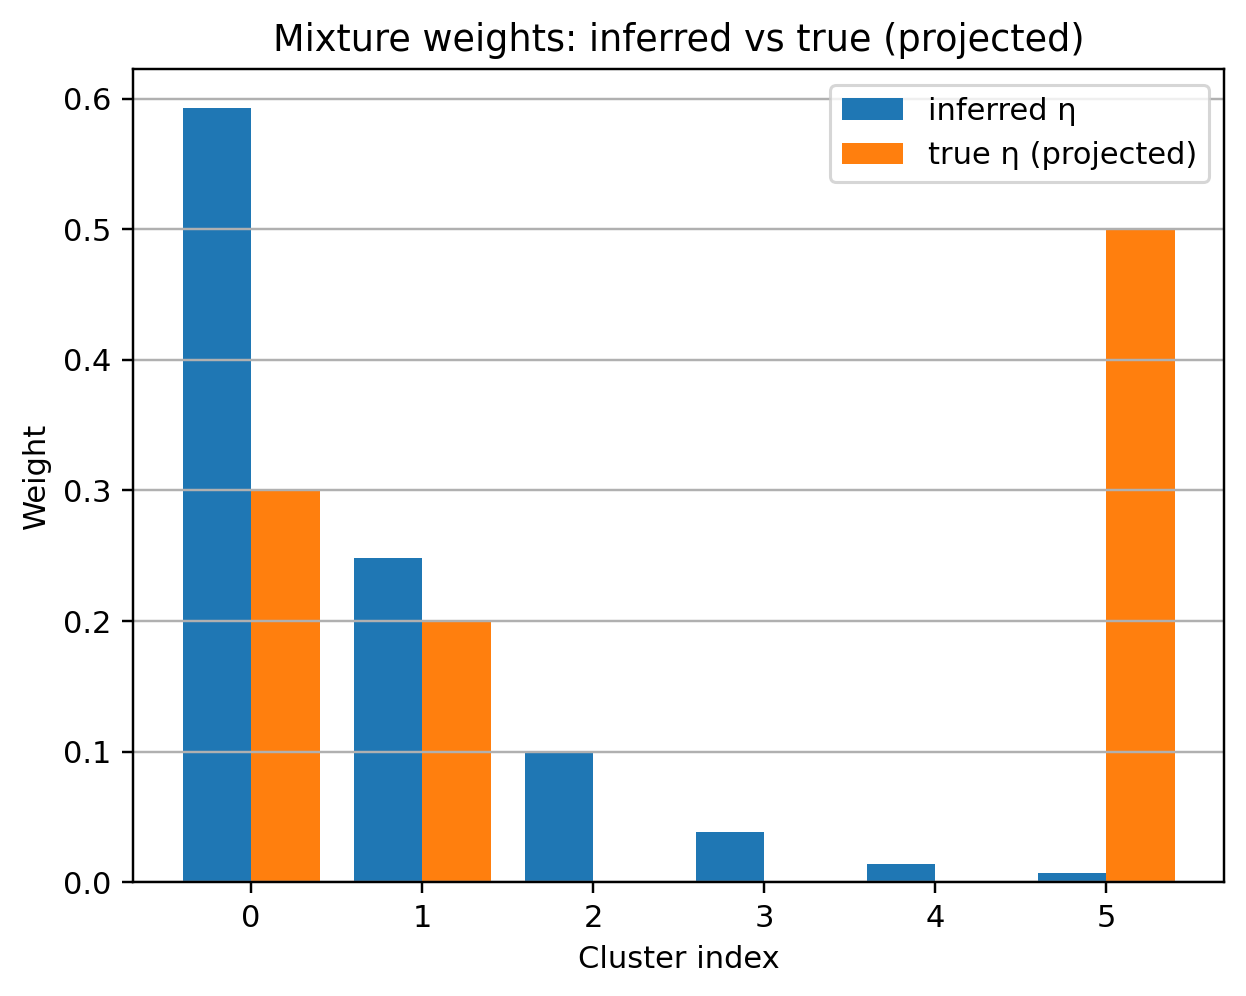}
  \caption{Inter}
\end{subfigure}\hfill
\caption{Mixture-weight calibration for persistent user for DTLZ dataset. Inter queries best match the true mixture, while random collapses to one mode and intra largely ignores 
$\eta$. Blue bars are inferred $\hat{\eta}$, orange bars are projected true $\eta^*$
via Hungarian alignment. (a) Random: blue mass on one index and orange-only bars → mode collapse. (b) Intra: blue focuses on one component → poor allocation across modes. (c) Inter: clear blue–orange alignment → best identification and calibration across modes}
\label{fig:metric3}
\end{figure*}

\begin{figure}
\centering
% First row
\begin{subfigure}{0.40\textwidth}
  \includegraphics[width=\linewidth]{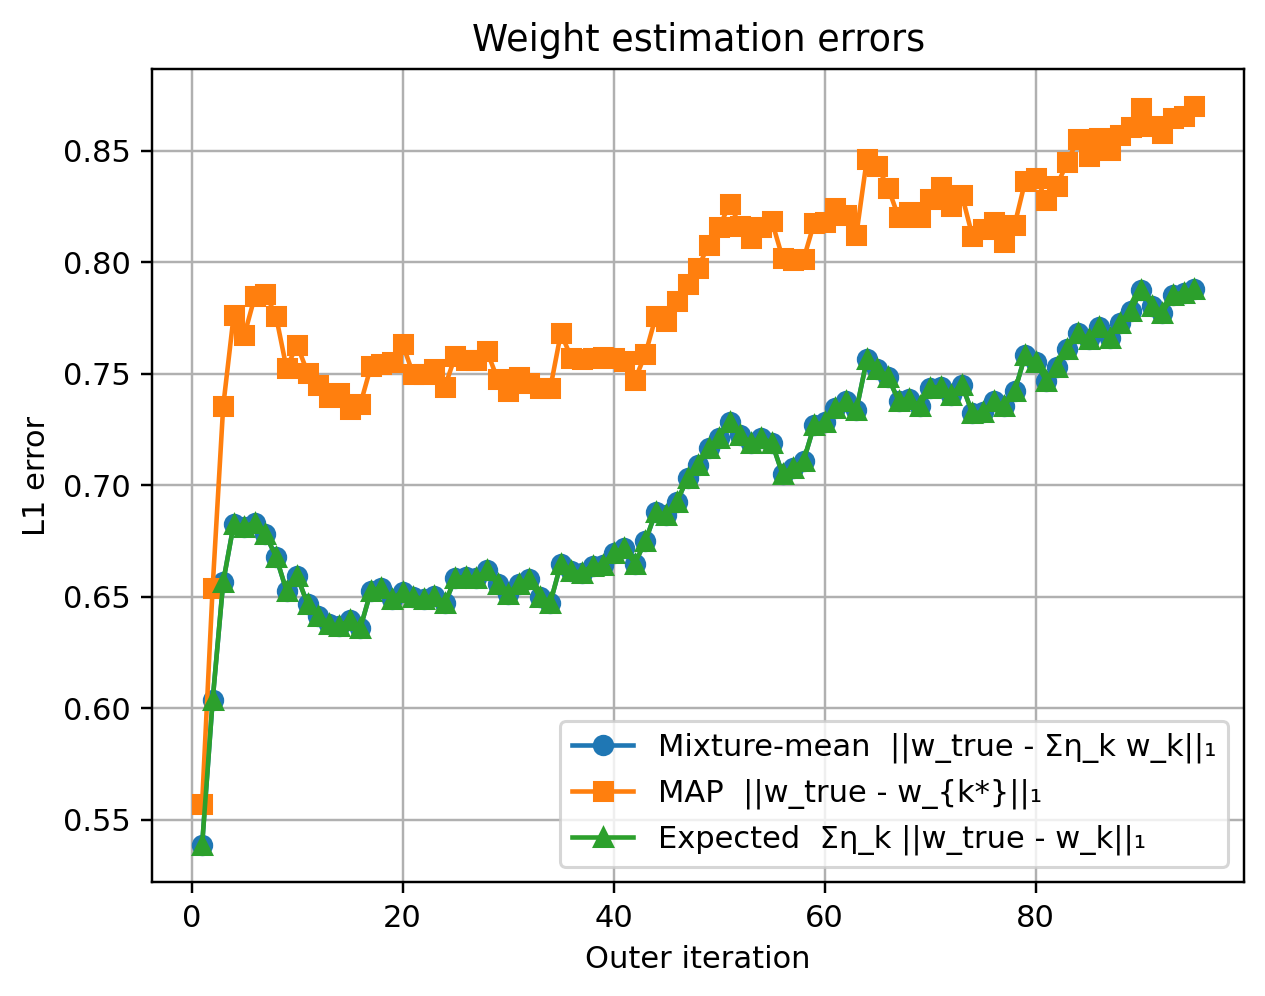}
  \caption{Clusterless}
\end{subfigure}\hfill
\begin{subfigure}{0.40\textwidth}
  \includegraphics[width=\linewidth]{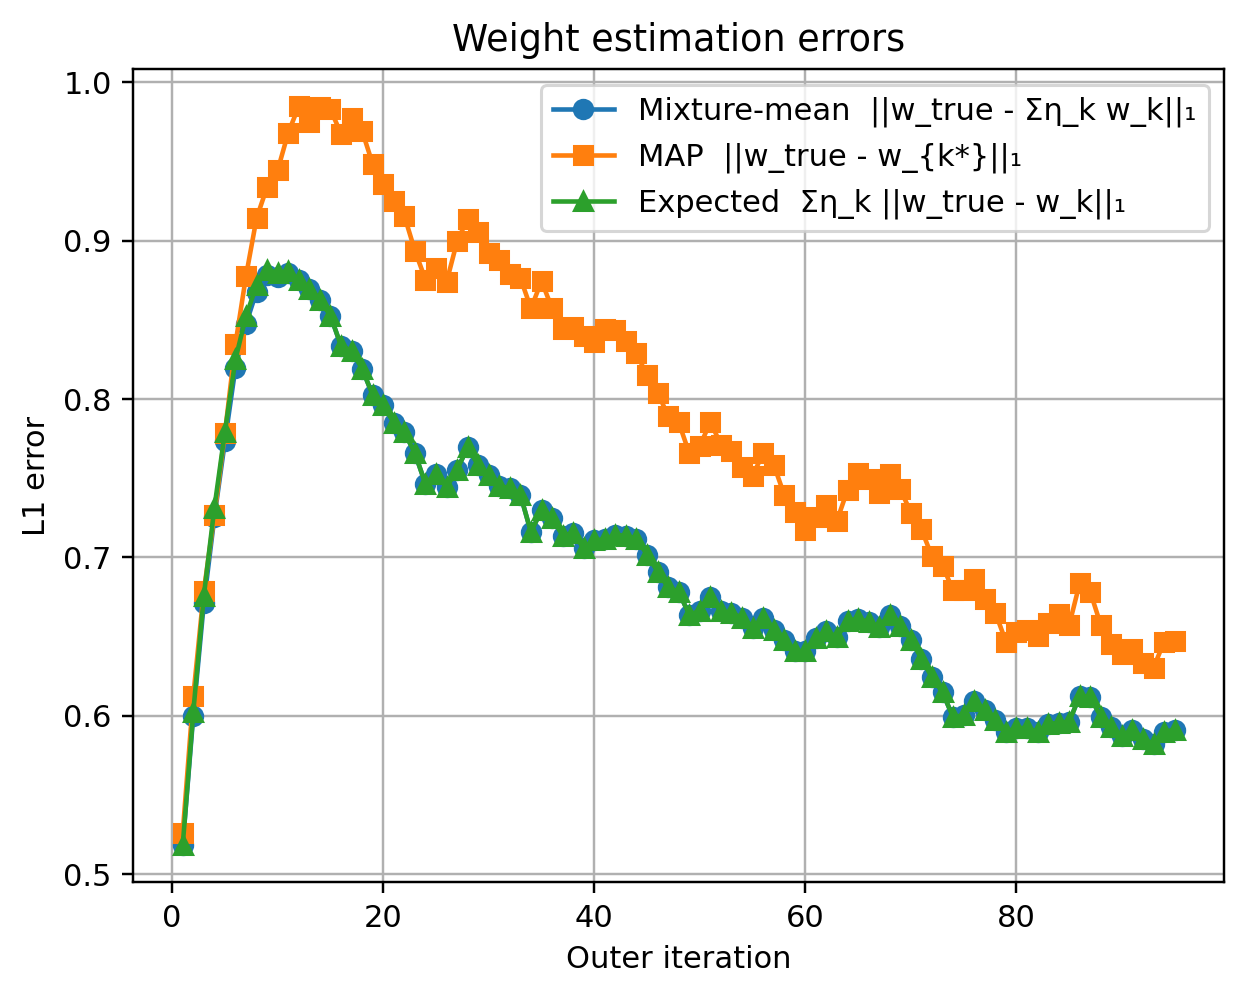}
  \caption{Inter}
\end{subfigure}
\caption{Errors of inferred preferences for persistent user for DTLZ dataset. Inter–queries quickly reduce mixture-mean and expected $L_1$ errors, while MAP improves more slowly; in contrast, clusterless drifts upward, reflecting entropy-only sampling under an averaged scalarizer and mode confusion. Curves: blue = mixture-mean $\mid \mid w_{true} - \sum_k \eta_k \bar{w}_k \mid \mid_1$, orange = MAP-cluster $\mid \mid w_{true} - \bar{w}_{k^*}\mid \mid$ with $k^* = \arg \max_k \eta_k$ and green = expected $\sum_k \eta_k  \mid \mid w_{true} - \bar{w}_k \mid \mid_1$. Lower is better.}
\label{fig:metric4}
\end{figure}

\begin{figure}
\centering
% First row
\begin{subfigure}{0.45\textwidth}
  \includegraphics[width=\linewidth]{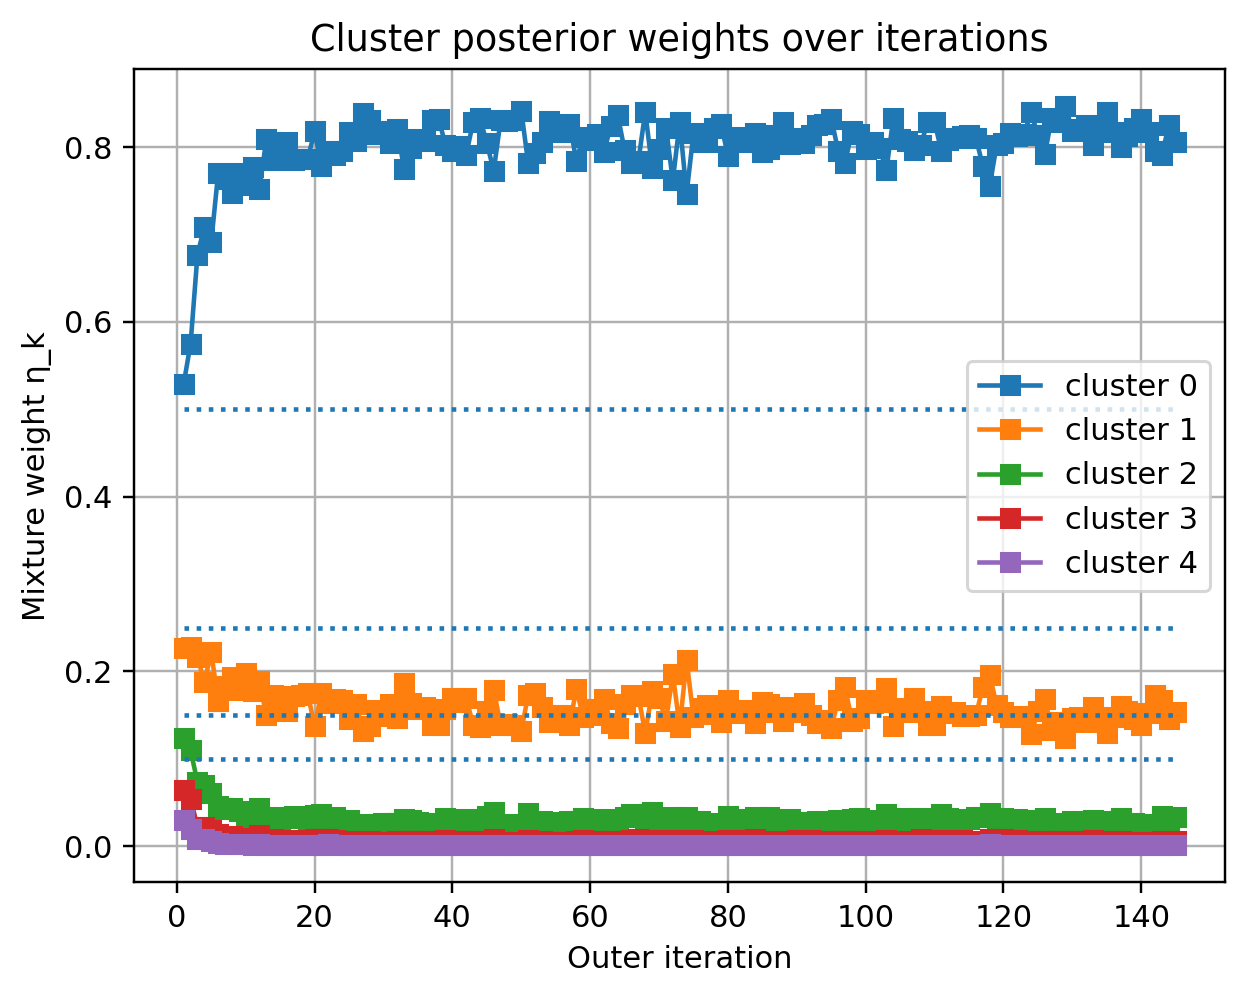}
  \caption{WFG dataset}
\end{subfigure}\hfill
\begin{subfigure}{0.45\textwidth}
  \includegraphics[width=\linewidth]{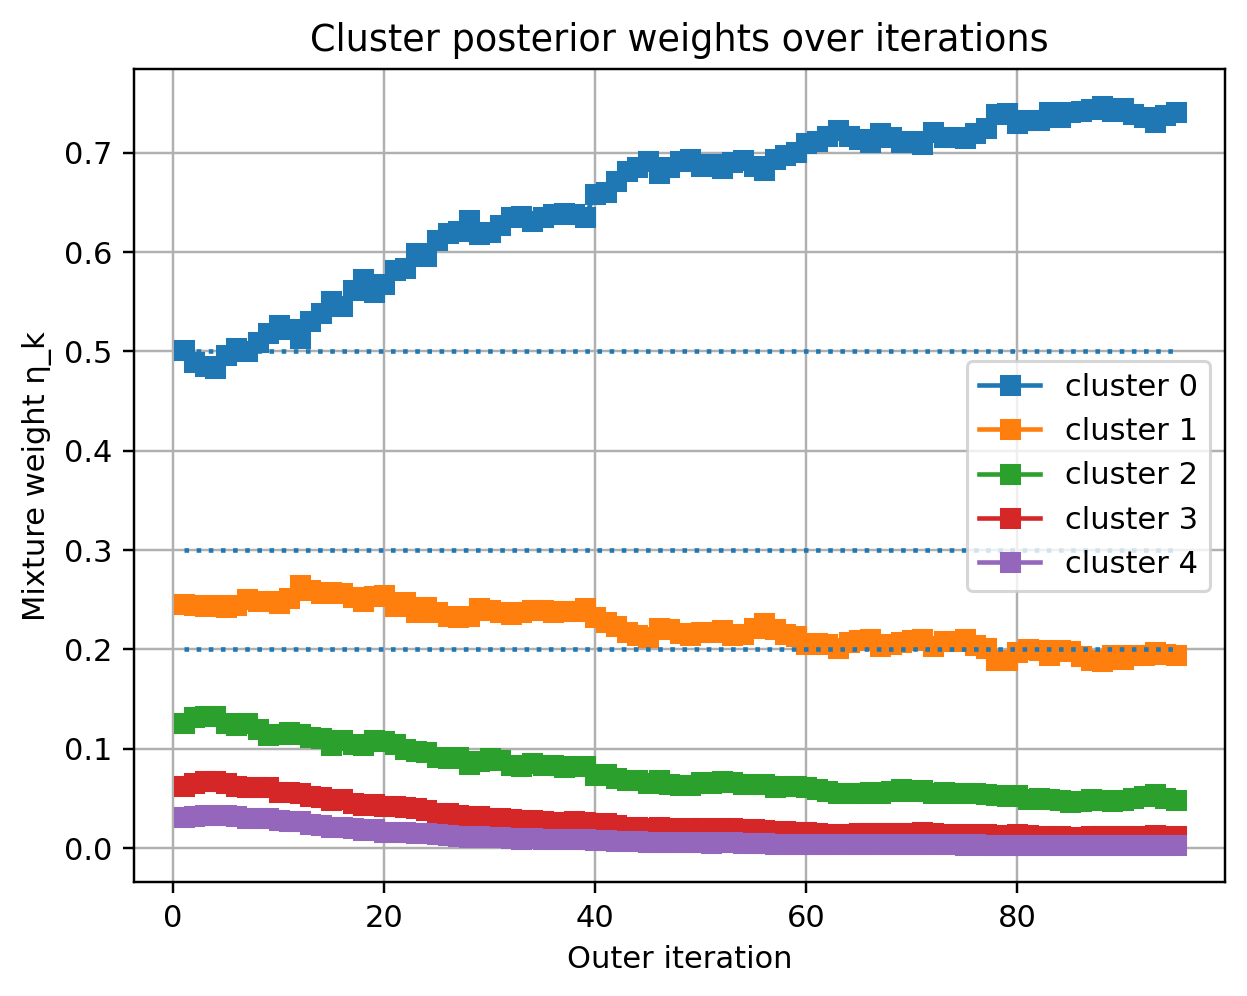}
  \caption{DTLZ dataset}
\end{subfigure}
\caption{Evolution of posterior mixture weights $\eta_k$ over outer iterations for WFG dataset}
\label{fig:posterior_mixture_weights}
\end{figure}

\begin{figure*}
\centering
% First row
\begin{subfigure}{0.33\textwidth}
  \includegraphics[width=\linewidth]{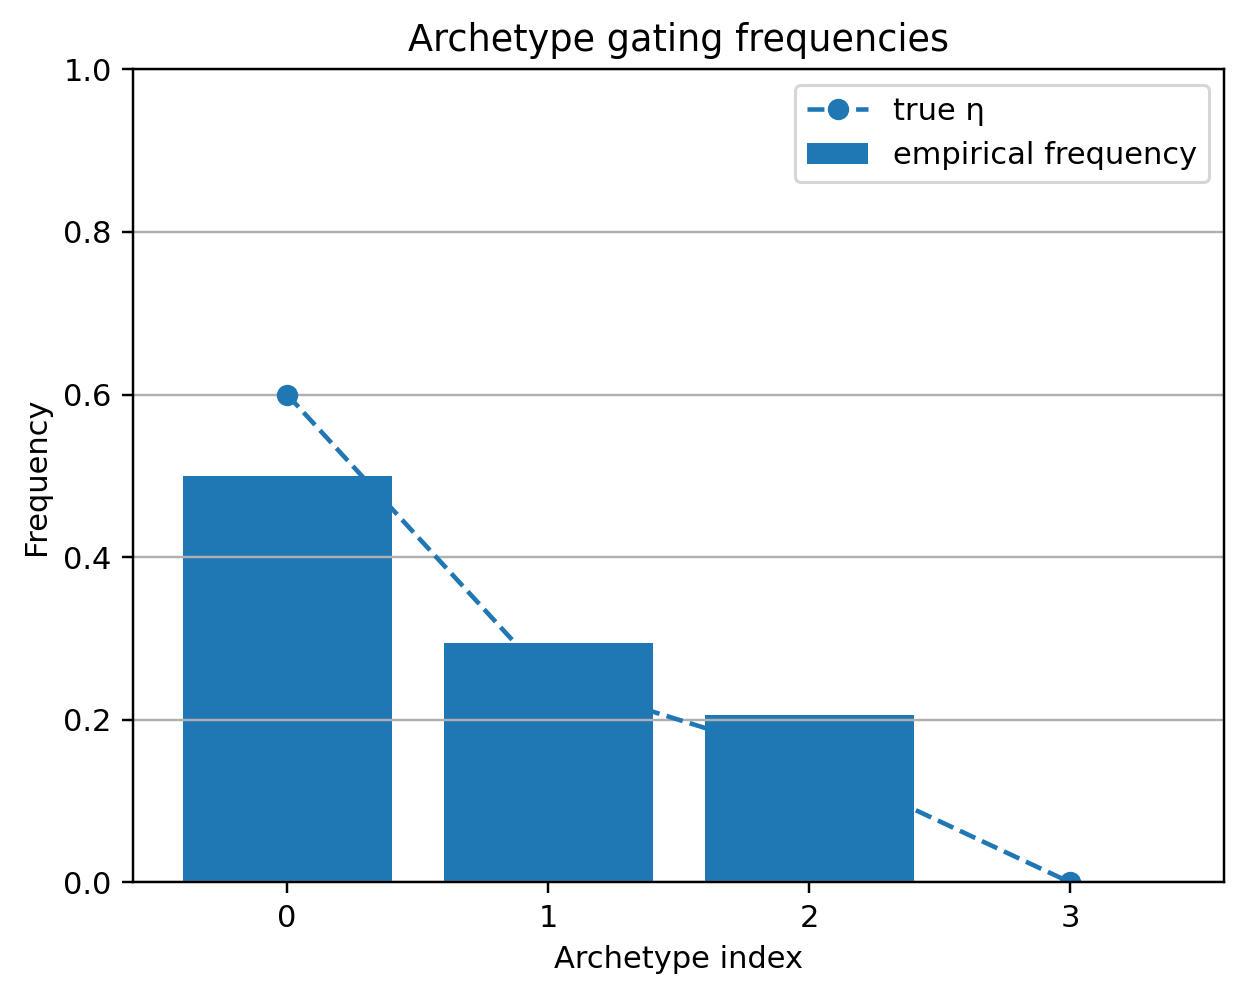}
  \caption{random}
\end{subfigure}\hfill
\begin{subfigure}{0.33\textwidth}
  \includegraphics[width=\linewidth]{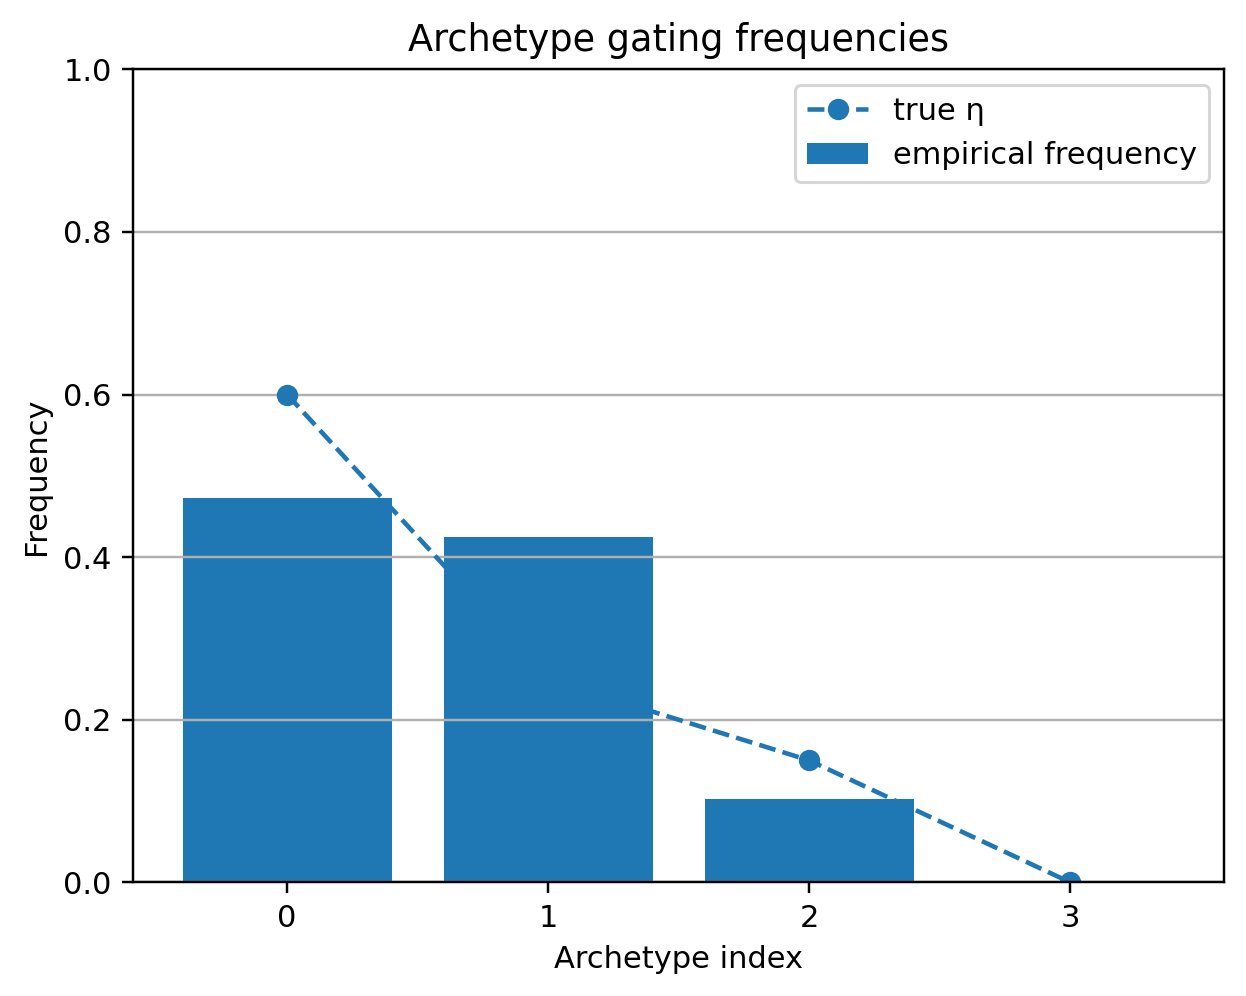}
  \caption{clusterless}
\end{subfigure}\hfill
\begin{subfigure}{0.33\textwidth}
  \includegraphics[width=\linewidth]{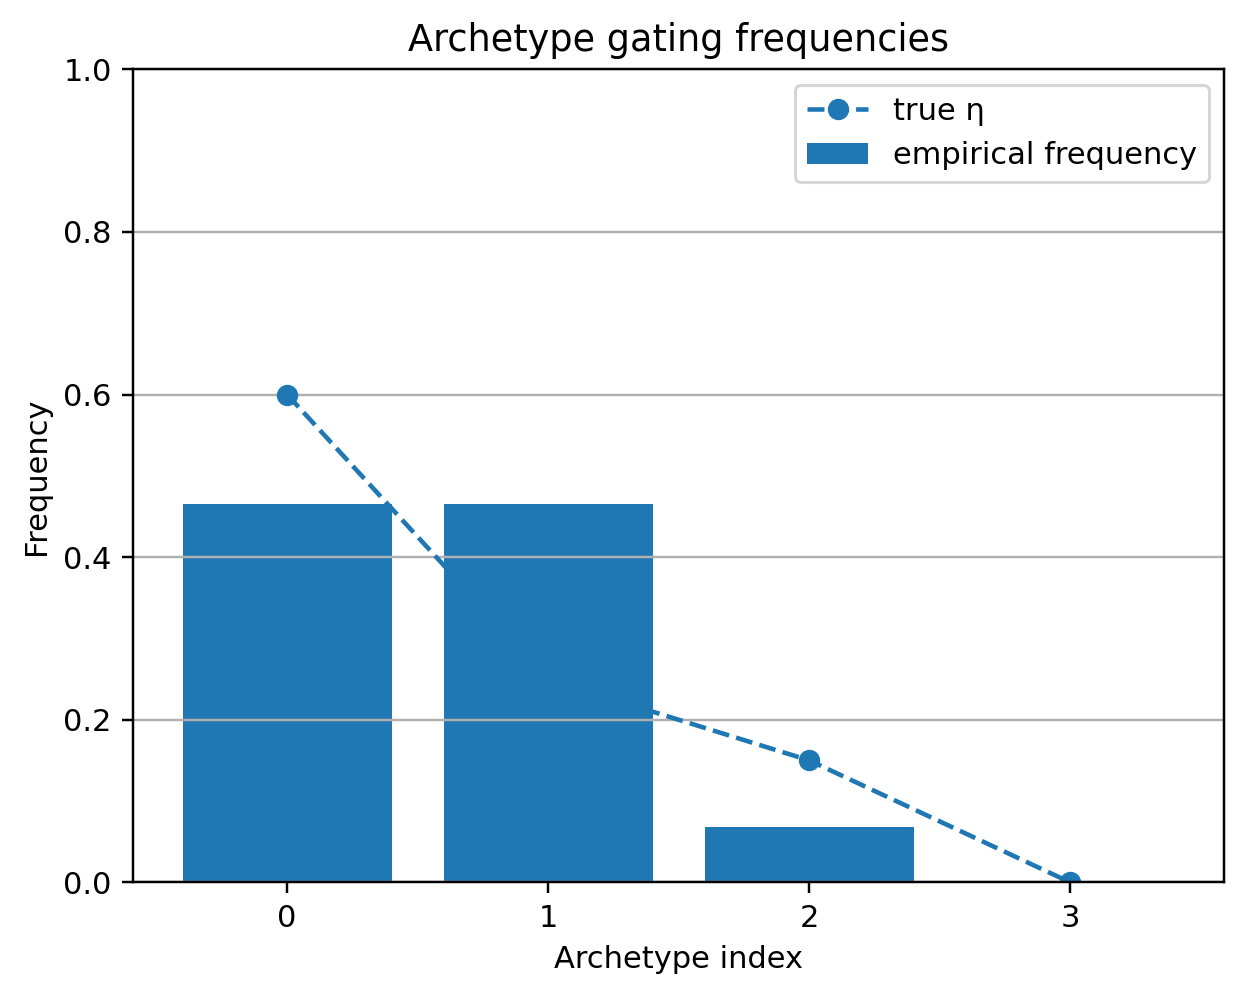}
  \caption{Intra}
\end{subfigure}\hfill
\begin{subfigure}{0.33\textwidth}
  \includegraphics[width=\linewidth]{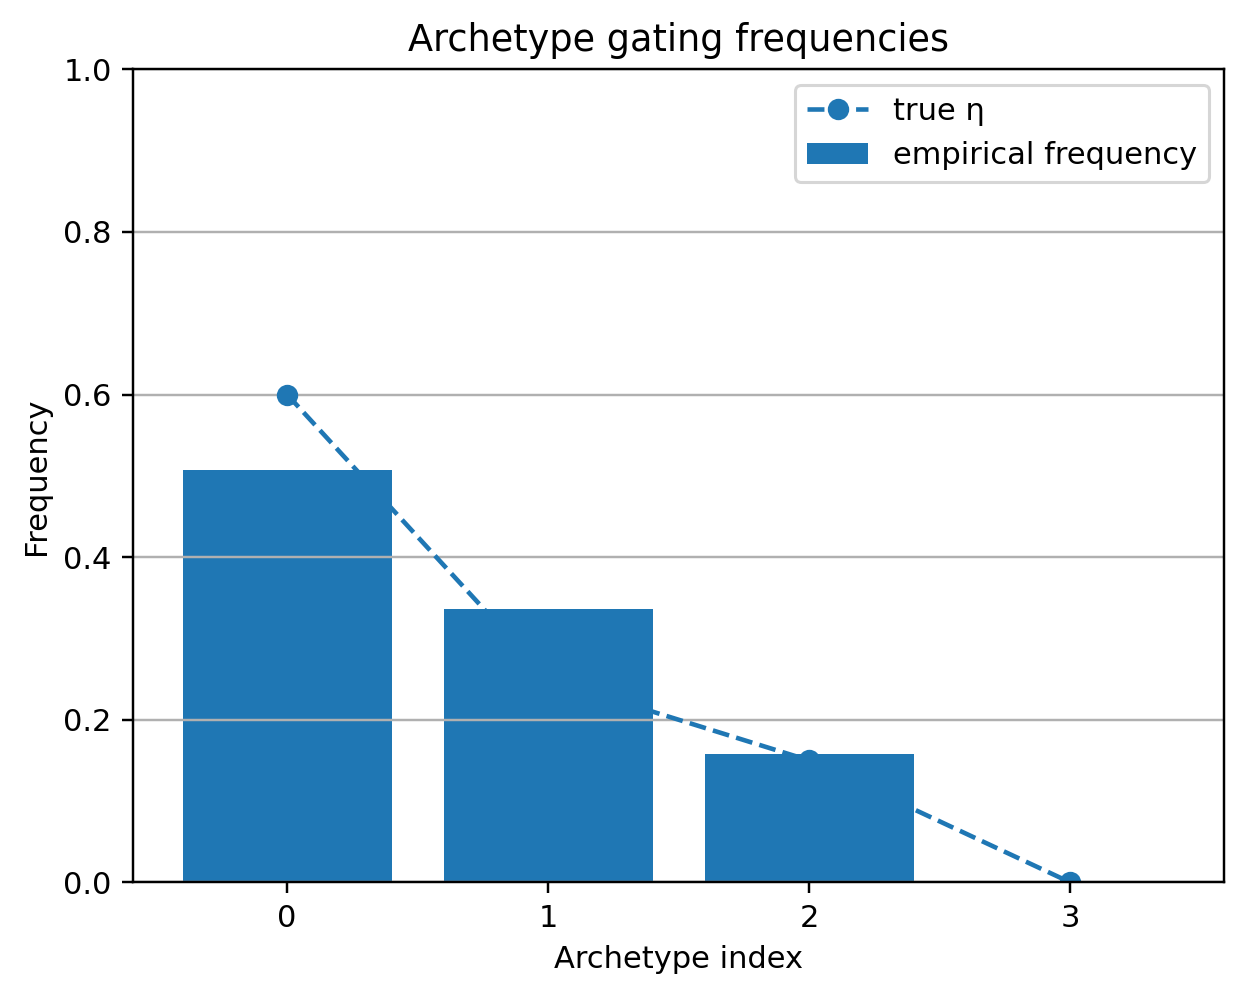}
  \caption{Inter}
\end{subfigure}\hfill
\begin{subfigure}{0.33\textwidth}
  \includegraphics[width=\linewidth]{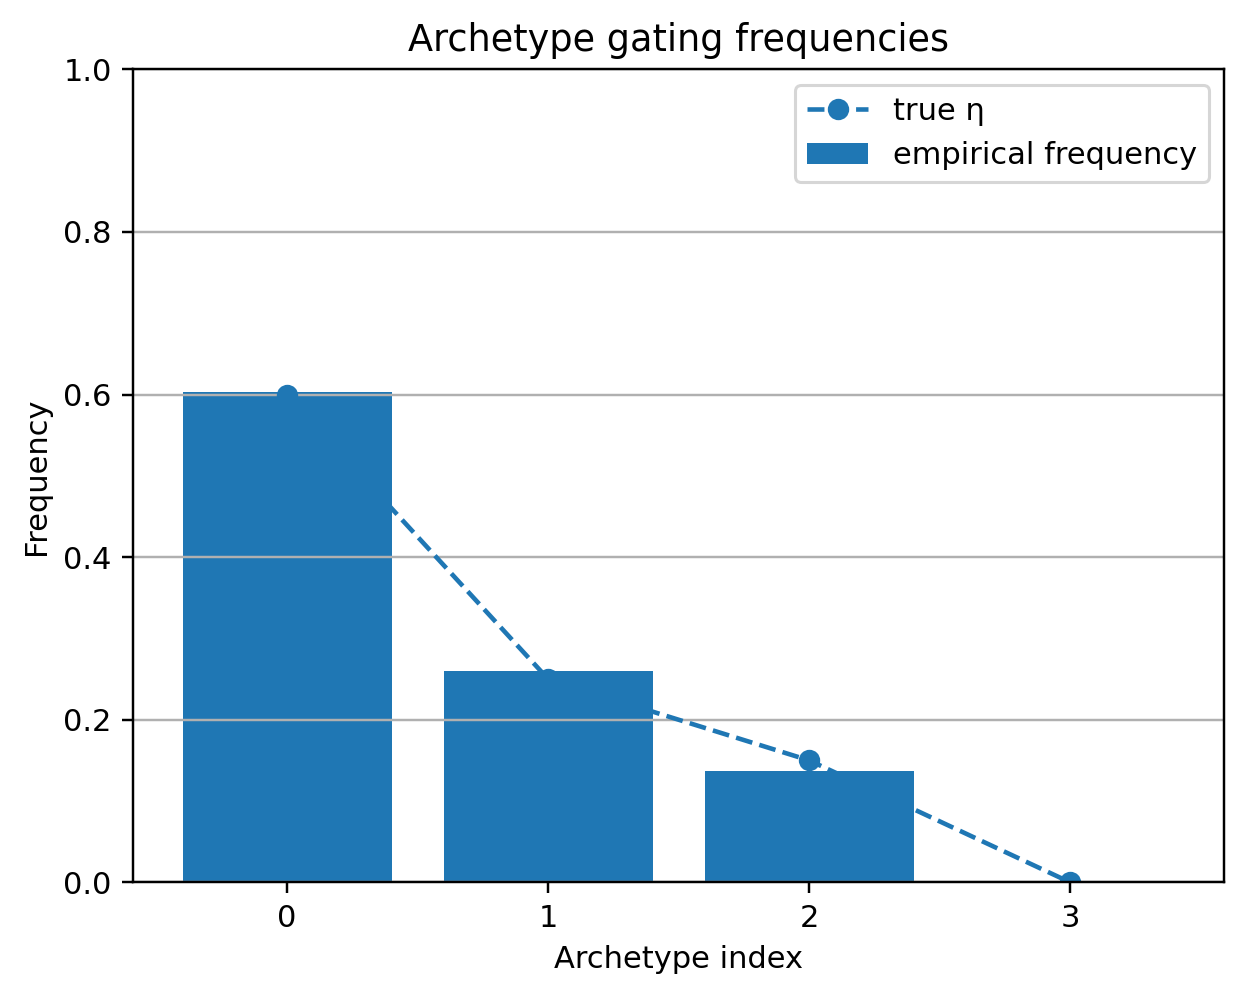}
  \caption{hybrid}
\end{subfigure}
\caption{Comparison of archetype-aware querying strategies (a–e) Empirical gating frequencies versus true mixture weights for different selection modes.
Hybrid scheduling achieves the closest alignment to the true mixture, demonstrating effective exploration across archetypes.}
\label{fig:gating_frequency}
\end{figure*}

The Figure \ref{fig:posterior_mixture_weights} shows posterior probability mass assigned to the cluster $k$ i.e. how model believes each archetype contributes to the overall mixture over series of iterations for WFG and DTLZ dataset. The query mode is hybrid in both cases. We can see for WFG dataset, cluster 0 dominates and rises to $\approx$ 0.7 and remains stable, cluster 1 is around $\approx 0.2$, cluster 2 and cluster 3 around 0.1 and cluster 4 around 0. This describes the true weights of WFG dataset as well ($\eta^\star=(0.50,\,0.25,\,0.15,\,0.10)$. The stabalization of weights happens roughly after 20 iterations. We can also see the plot for DTLZ dataset. For DTLZ dataset, we can see that cluster 0 dominates and rises to $\approx$ 0.7, cluster 1 is around 0.2, cluster 2 is around 0.1 and cluster 3,4 are around 0. This is also close to DTLZ \(\eta^\star=(0.5,0.3,0.2)\). 

The Figure \ref{fig:posterior_mixture_weights} shows posterior probability mass assigned to the cluster $k$ i.e. how model believes each archetype contributes to the overall mixture over series of iterations for WFG and DTLZ dataset. The query mode is hybrid in both cases. We can see for WFG dataset, cluster 0 dominates and rises to $\approx$ 0.7 and remains stable, cluster 1 is around $\approx 0.2$, cluster 2 and cluster 3 around 0.1 and cluster 4 around 0. This describes the true weights of WFG dataset as well ($\eta^\star=(0.50,\,0.25,\,0.15,\,0.10)$. The stabalization of weights happens roughly after 20 iterations. We can also see the plot for DTLZ dataset. For DTLZ dataset, we can see that cluster 0 dominates and rises to $\approx$ 0.7, cluster 1 is around 0.2, cluster 2 is around 0.1 and cluster 3,4 are around 0. This is also close to DTLZ \(\eta^\star=(0.5,0.3,0.2)\).

Figure \ref{fig:gating_frequency} gating-frequency panels (a–e) show how each policy allocates queries among latent preference archetypes, while the regret plot (f) shows the impact of that allocation on optimization performance.
Random and clusterless ignore mixture structure; intra collapses to one mode; inter balances but lacks fine exploitation; hybrid balances exploration across archetypes and exploitation within them—achieving both accurate mixture recovery and lowest regret.

% \begin{figure}
% \centering
% % First row
% \begin{subfigure}{0.45\textwidth}
%   \includegraphics[width=\linewidth]{Results/wfgResults/MixtureWeights/clusterless_plot_eta_vs_true.png}
%   \caption{Clusterless}
% \end{subfigure}\hfill
% \begin{subfigure}{0.45\textwidth}
%   \includegraphics[width=\linewidth]{Results/wfgResults/MixtureWeights/clusterless_plot_eta_vs_true.png}
%   \caption{Hybrid}
% \end{subfigure}
% \caption{Mixture-weight calibration for persistent user for WFG dataset. We can see samples from clusterless query versus hybrid query.}
% \label{fig:metric5}
% \end{figure}

% \bibliography{uai2026-template/uai2026-template}
% \end{document}
